# Supplementary material for: Learning to Explore Informative Trajectories and Samples for Embodied Perception
Source: arXiv:2303.10936 source file (2023-03-20)
Supplement: Supplementary file 1 [file 070appendix.tex]

\section{\color{red}Learning Curves}
To fairly compare with previous methods, we set the number of training steps to 500k in all experiments. The learning curves are shown in Fig.~\ref{fig:loss}. We save the best model according to the reward value. It can be seen that two methods obtain the best model when training about 320k steps. 

\section{Detection Performances on the Learned Trajectories}

To further demonstrate the effectiveness of our exploration policy, we compare the detection performances on the learned trajectories by different methods shown in Tab.~\ref{tab:tra}. It can be seen that the pre-trained perception model obtains the worst performance on our trajectories. Since these images are more difficult to perceive, utilizing them to fine-tune the perception model can make it generalize better to the unseen 3D environment. 

\begin{figure}[t]
\centering
\includegraphics[width=0.95\linewidth]{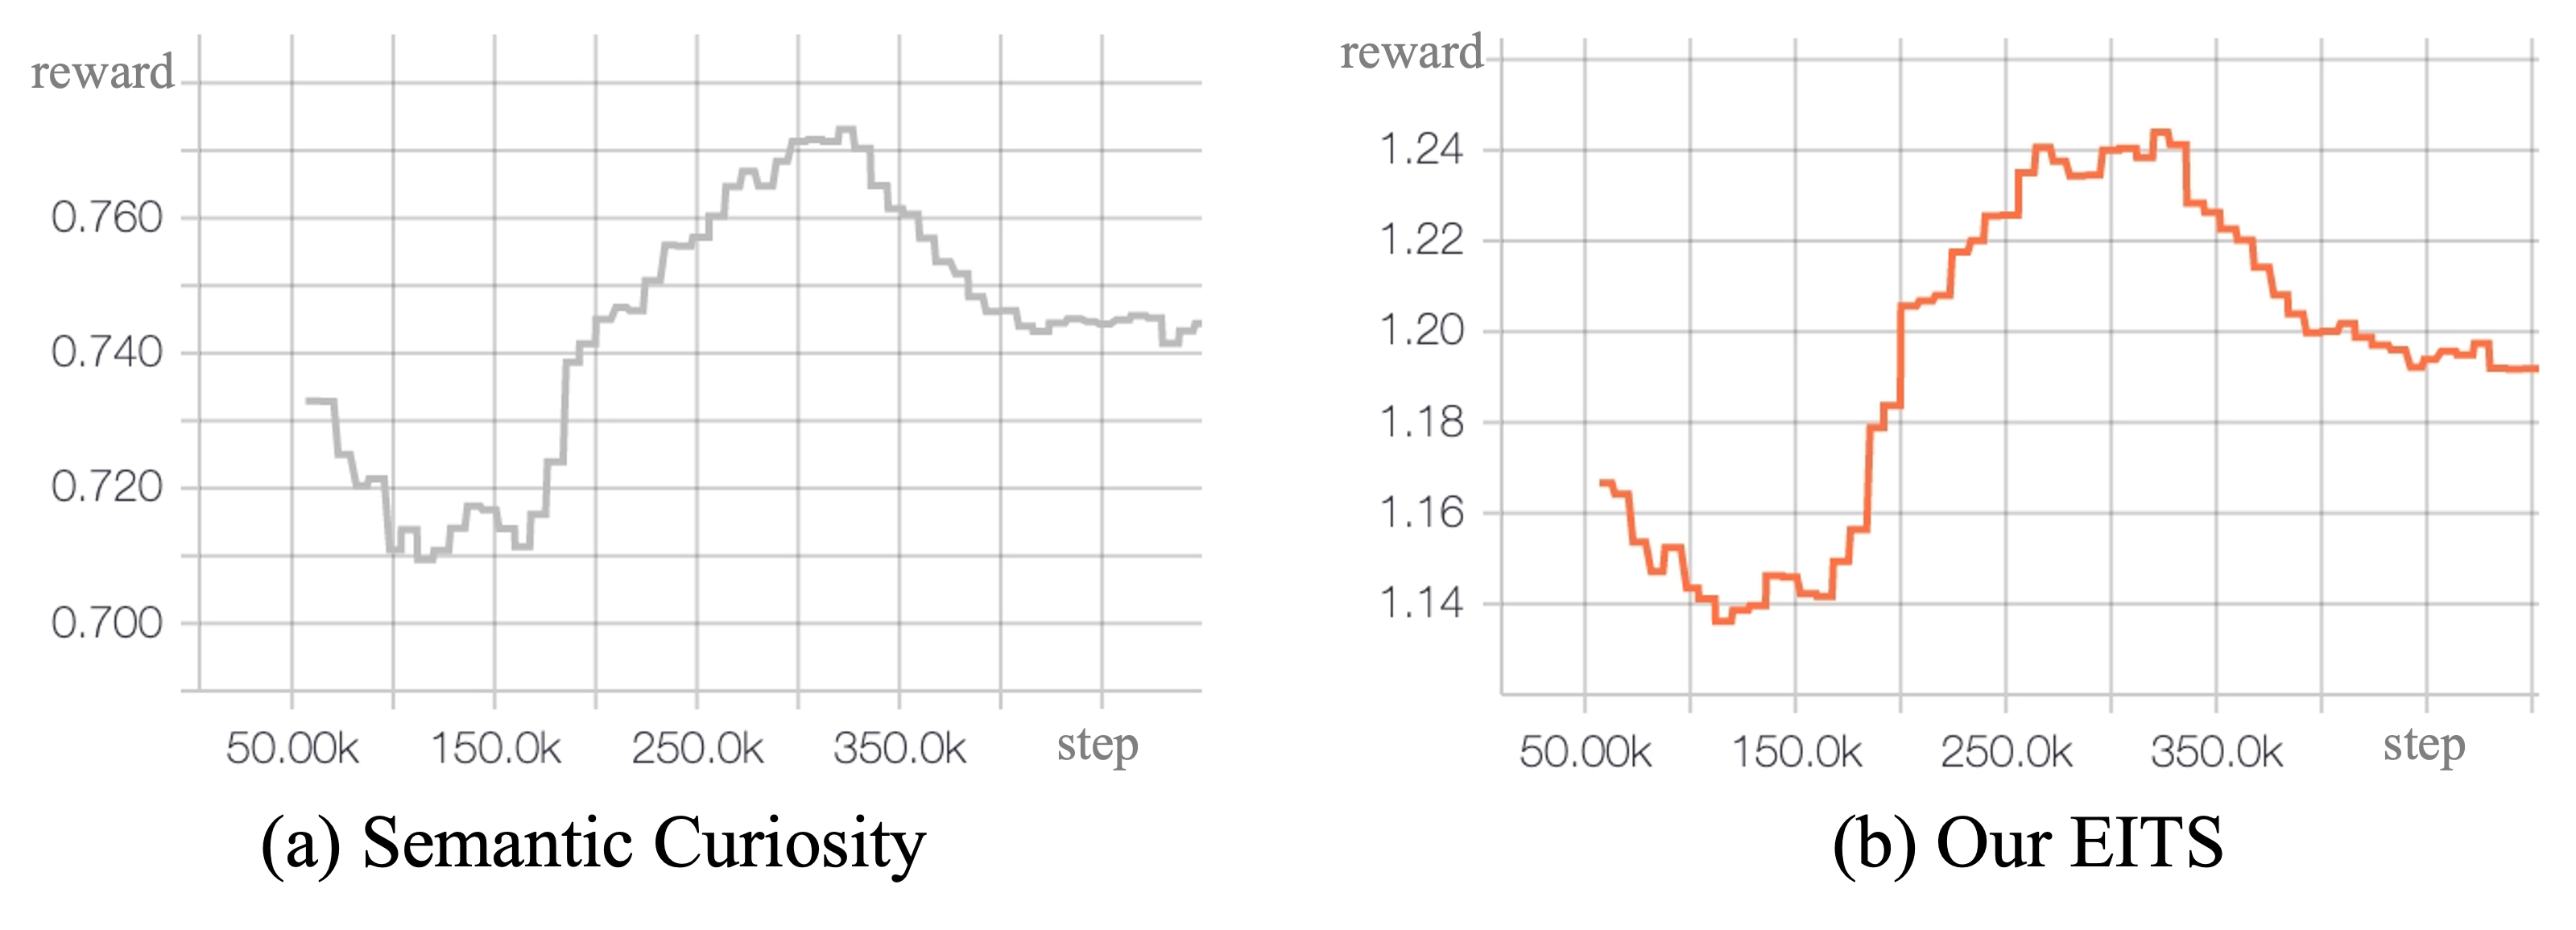}
\caption{The learning curves of two methods (i.e., Semantic Curiosity and Our EITS). The ‘reward’ means the average of the episode reward, which is a queue of length 1000. }
\label{fig:loss}
\end{figure}

\begin{table}[h]
\caption{The performance of the pre-trained object detection model on the explored trajectories.}
\label{tab:tra}
\resizebox{\linewidth}{!}{
\begin{tabular}{l|cccccc|c}
\hline
{Method}&{Chair}&{Couch}&{Potted Plant}&{Bed}&{Toilet}&{Tv}&{Average} \\
\hline
{Random}&{23.31}&{27.30}&{9.36}&{23.05}&{4.32}&{17.23}&{17.42}\\
{Active Neural SLAM \cite{chaplot2020learning}}&{18.18}&{23.60}&{10.86}&{18.62}&{13.32}&{6.94}&{15.25}\\
{Semantic Curiosity \cite{chaplot2020semantic}}&{18.56}&{17.57}&{10.88}&{18.38}&{11.49}&{8.44}&{14.22}\\
{Ours}&{17.74}&{18.78}&{8.41}&{17.59}&{10.43}&{7.51}&{\bf{13.42}}\\
\hline
\end{tabular}
}
\end{table}
